# Supplementary material for: Probing and Fine-tuning Reading Comprehension Models for Few-shot Event Extraction
Source: arXiv:2010.11325 source file (2020-10-21)
Supplement: Supplementary file 1 [file appendix.tex]

\section{Appendix}

\subsection{Experiment settings}
